# Supplementary material for: Nighttime Smartphone Reflective Flare Removal Using Optical Center Symmetry Prior
Source: arXiv:2303.15046 source file (2023-03-27)
Supplement: Supplementary file 2 [file Supp_fig3.pdf]

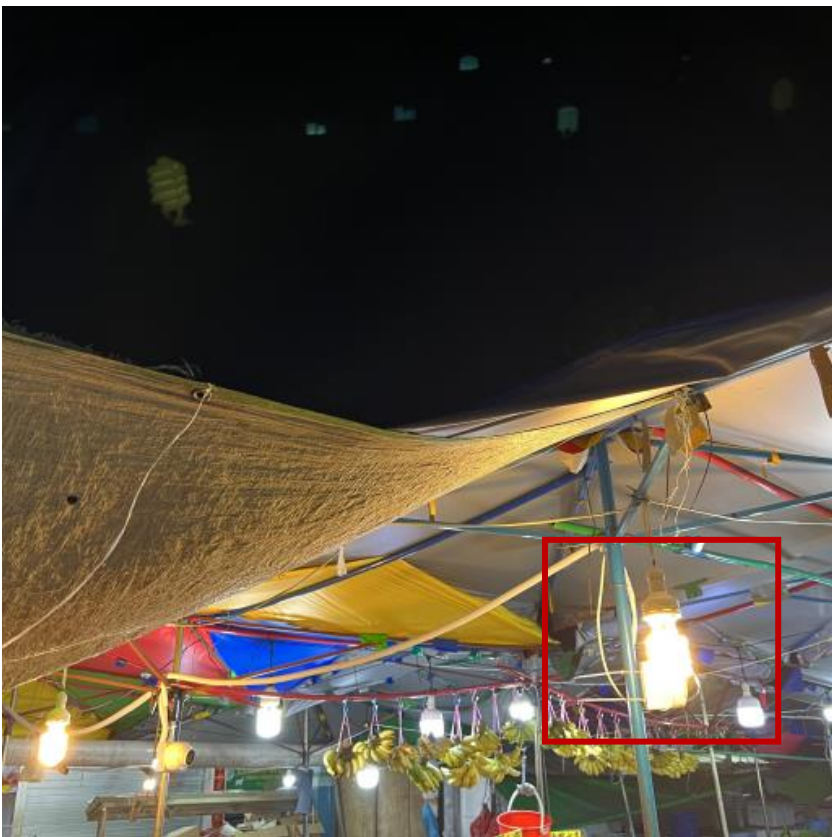

(a) Before single-shot HDR

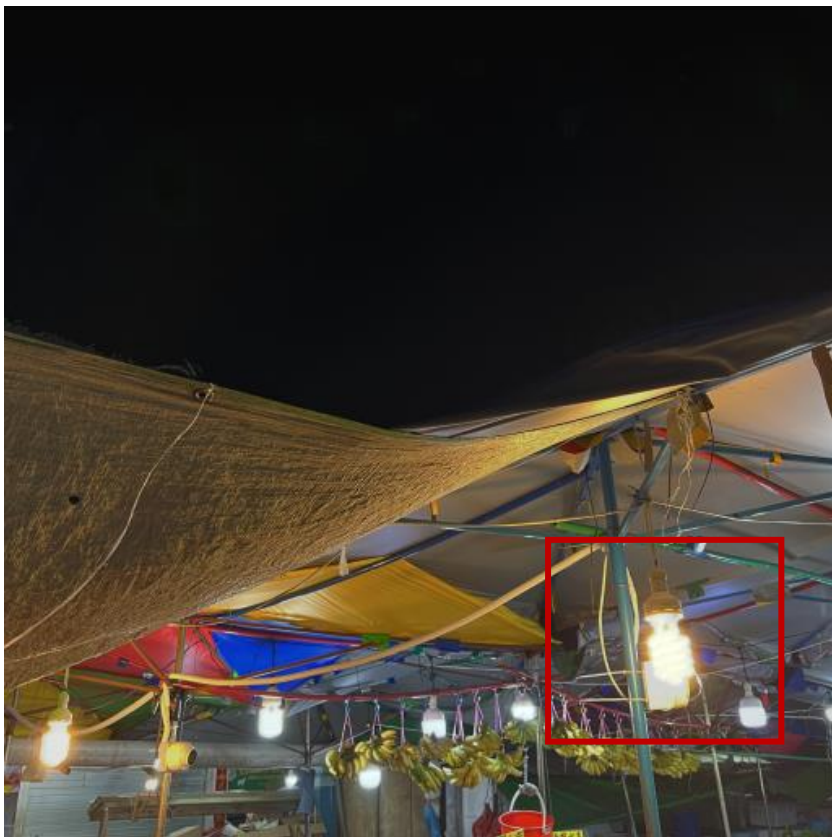

(b) After single-shot HDR

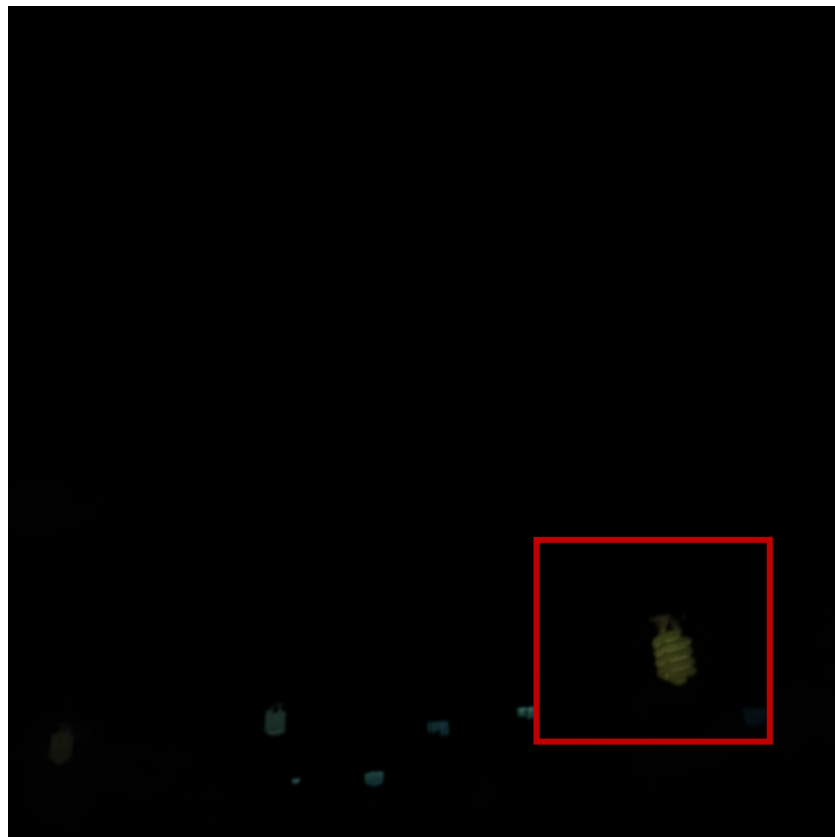

(c) Estimated flare

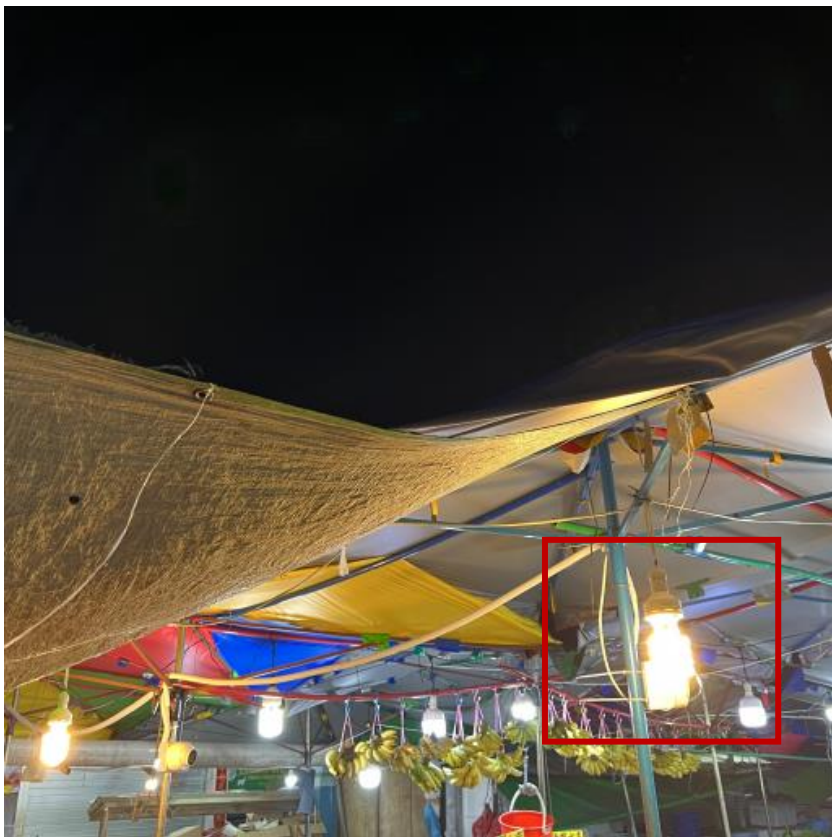

(a) Before single-shot HDR

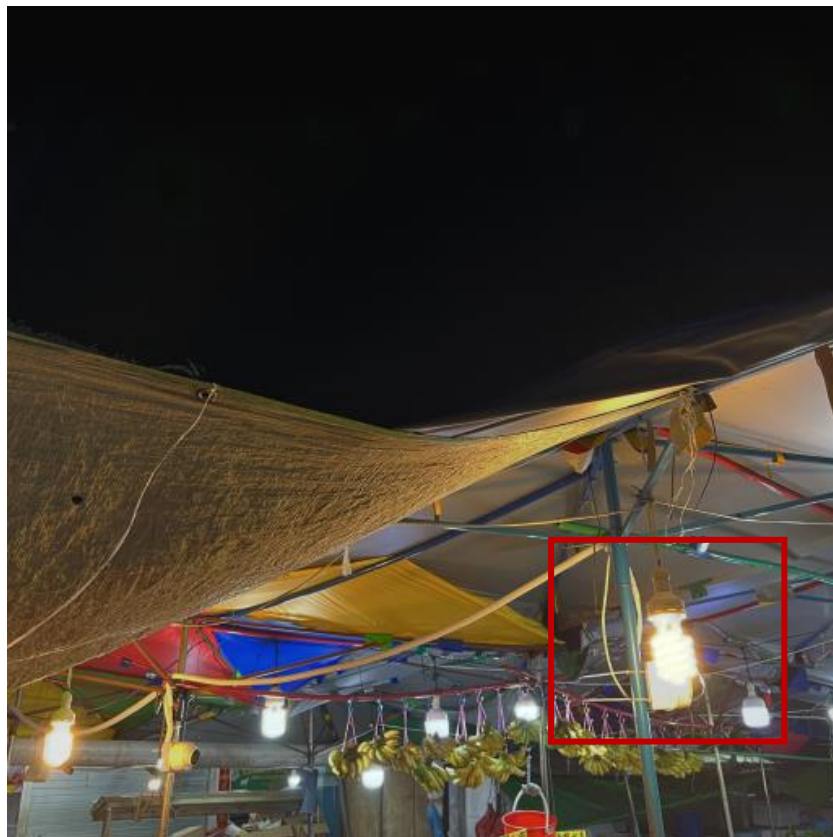

(b) After single-shot HDR

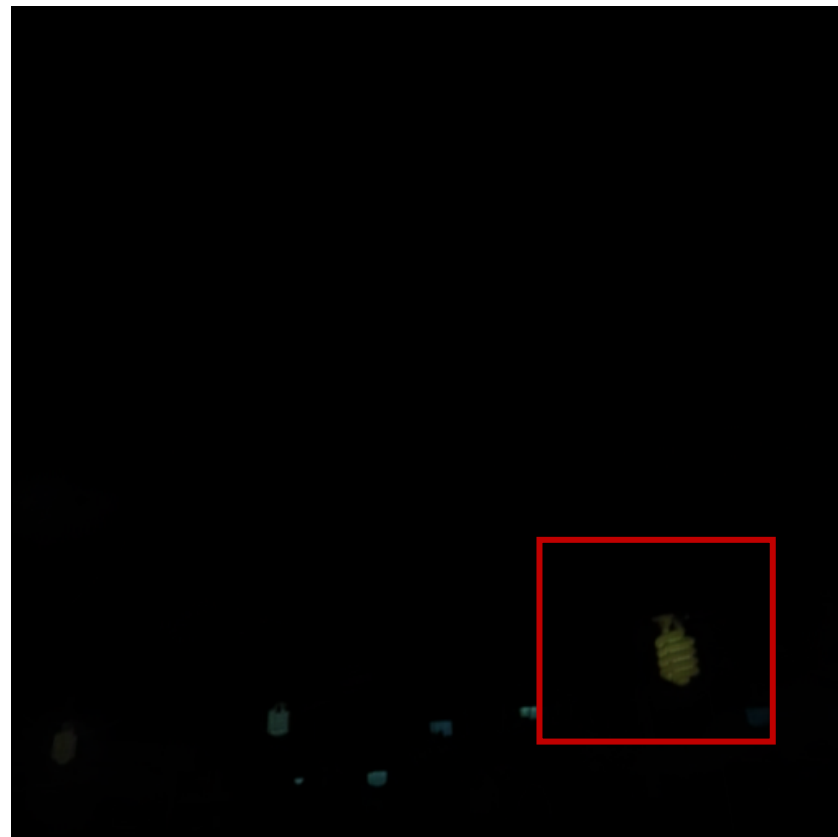

(c) Estimated flare
